# Supplementary material for: Superconducting Fluctuations in the Normal State of the Two-Dimensional Hubbard Model
Source: arXiv:1507.04475 source file (2015-09-14)
Supplement: Supplementary file 1 [file supplemental.pdf]

# Supplemental material for: Superconducting Fluctuations in the Normal State of the Two-Dimensional Hubbard Model

Xi Chen,[1] J. P. F. LeBlanc,[1] and Emanuel Gull[1]
[1]*Department of Physics, University of Michigan, Ann Arbor, Michigan 48109, USA*
(Dated: September 14, 2015)

## SUSCEPTIBILITIES AND CORRELATED PAIRING SUSCEPTIBILITY

We define the one-particle and two-particle Green's functions in imaginary time, $\tau$ as

$$G_\sigma(k_1\tau_1, k_2\tau_2) = \langle T_\tau(c^\dagger_{k_1\sigma}(\tau_1)c_{k_2\sigma}(\tau_2)\rangle \tag{1}$$

$$G_{2,\sigma_1\sigma_2\sigma_3\sigma_4}(k_1\tau_1, ..., k_4\tau_4) = \langle T_\tau(c^\dagger_{k_1\sigma}(\tau_1)c_{k_2\sigma}(\tau_2)c^\dagger_{k_3\sigma}(\tau_3)c_{k_4\sigma}(\tau_4)\rangle. \tag{2}$$

We operate in a formalism which allows for a non-zero anomalous Green's function, in the superconducting state which is defined as

$$F(k,\tau) = -\langle T_\tau c_{k\uparrow}(\tau)c_{-k\downarrow}(0)\rangle. \tag{3}$$

The generalized susceptibility can be written in imaginary time, $\tau$, in terms of the one- and two-particle Green's functions as[1]

$$\chi_{\sigma_1\sigma_2\sigma_3\sigma_4}(k_1\tau_1, k_2\tau_2, k_3\tau_3, k_4\tau_4) = G_{2,\sigma_1...\sigma_4}(k_1\tau_1, k_2\tau_2, k_3\tau_3, k_4\tau_4) - G_{\sigma_1\sigma_2}(k_1\tau_1, k_2\tau_2)G_{\sigma_3\sigma_4}(k_3\tau_3, k_4\tau_4).$$

The susceptibility can be represented in frequency space via a Fourier transform. In the particle-particle (pp) convention, it is defined as

$$\chi^{\omega\omega'\nu}_{pp\sigma\sigma'}(k,k',q) = \int_0^\beta\int_0^\beta\int_0^\beta d\tau_1 d\tau_2 d\tau_3 \chi_{\sigma\sigma\sigma'\sigma'}(k\tau_1, (q-k')\tau_2, (q-k)\tau_3, k'0) \times e^{-i\omega\tau_1}e^{i(\nu-\omega')\tau_2}e^{-i(\nu-\omega)\tau_3}$$

where $\omega$ and $\omega'$ are fermionic Matsubara frequencies, $\nu$ is a bosonic Matsubara frequency, $\sigma$ and $\sigma'$ are $\uparrow$ or $\downarrow$ spin labels and $k$, $k'$ and $q$ are initial, final and transfer momenta respectively. We define the difference between the $\sigma\sigma' \equiv \uparrow\uparrow$ and $\uparrow\downarrow$ susceptibilities as

$$\chi_{pp\overline{\uparrow\downarrow}} = \chi_{pp\uparrow\uparrow} - \chi_{pp\uparrow\downarrow}. \tag{4}$$

One can show that $\chi_{pp\overline{\uparrow\downarrow}}$ is directly related to the superconducting state using linear response theory where we obtain

$$\sum_{kk'\omega\omega'} \chi^{\omega\omega'\nu=0}_{pp\overline{\uparrow\downarrow}}(k,k',q=0)g(k)g(k') = \int_0^\beta d\tau' \sum_{kk'} \frac{\delta F(k,\tau=0;\eta)}{\delta\eta(k',\tau')} g(k)g(k')\bigg|_{\eta=0} \tag{5}$$

where $\eta$ is the strength of an external superconducting field and $F(k,\tau;\eta)$ is the anomalous Green's function with the existence of an external field. $g(k)$ is any symmetry function.

In general, the anomalous Green's function relates directly to the superconducting order parameter and is obtained via

$$F(k,\tau;\eta) = -\langle T_\tau c_{k\uparrow}(\tau)c_{-k\downarrow}(0)\rangle_\eta = -\frac{Tr\{e^{-\beta H}T_\tau[Sc_{k\uparrow}(\tau)c_{-k\downarrow}(0)]\}}{Tr(e^{-\beta H}T_\tau S)}. \tag{6}$$

where $H$ is the original Hamiltonian without source and

$$S = \exp[-\int_0^\beta d\tau' \sum_{k'} \left( c_{-k'\downarrow}(\tau') c_{k'\uparrow}(\tau') + c^\dagger_{k'\uparrow}(\tau') c^\dagger_{-k'\downarrow}(\tau') \right) \eta(k', \tau')]. \tag{7}$$

In order to obtain the susceptibility of a desired symmetry, the corresponding form factor is multiplied to $\chi_{pp\overline{\uparrow\downarrow}}$.[2]
This is the same quantity as the uniform pairing susceptibility defined in Ref. [3],

$$\begin{aligned}\chi^\alpha &= \frac{1}{N}\int_0^\beta d\tau \langle \sum_i \Delta_i^\alpha(\tau) \sum_j \Delta_j^\alpha(0) \rangle \\ &= \frac{1}{N}\int_0^\beta d\tau \langle \frac{1}{4} \sum_{mm'ij} f_{im} f_{jm'} \left( c_{i\uparrow} c_{m\downarrow} c^\dagger_{m'\downarrow} c^\dagger_{j\uparrow} - c_{i\uparrow} c_{m\downarrow} c^\dagger_{m'\uparrow} c^\dagger_{j\downarrow} - c_{i\downarrow} c_{m\uparrow} c^\dagger_{m'\downarrow} c^\dagger_{j\uparrow} + c_{i\downarrow} c_{m\uparrow} c^\dagger_{m'\uparrow} c^\dagger_{j\downarrow} \right) \rangle,\end{aligned} \tag{8}$$

where $f_{ij}$ is the symmetry factor in real space. For example, $f_{ij} = \delta_{ij}$ for $s$-wave; for $d$-wave $f_{ij} \neq 0$ if $i$ and $j$ are nearest neighbors and $j > i$; if the bond is along $x$ axis $f_{ij} = 1$, otherwise $f_{ij} = -1.\Delta_i(\tau)$ is the pairing parameter defined as

$$\Delta_i(\tau) = \frac{1}{2}\sum_j f^\alpha_{ij} e^{\tau H} (c_{i\uparrow} c_{j\downarrow} - c_{i\downarrow} c_{j\uparrow}) e^{-\tau H}. \tag{9}$$

We define the bare susceptibility,

$$\chi^{\omega\omega'\nu}_{0pp}(k, k', q) = -\beta G_\sigma(k, i\omega) G_\sigma(q - k', i\nu - i\omega') \delta_{\omega\omega'} \delta_{kk'}, \tag{10}$$

where the spin index on the left hand side has been omitted when we restrict our calculation to the paramagnetic state. The Bethe-Salpeter equation in this channel is [1]

$$\chi^{\omega\omega'\nu}_{pp\overline{\uparrow\downarrow}}(k, k', q) = \chi^{\omega\omega'\nu}_{0pp}(k, k', q) - \frac{1}{\beta^2} \chi^{\omega\omega''\nu}_{pp\overline{\uparrow\downarrow}}(k, k'', q) \Gamma^{\omega''\omega'''\nu}_{pp\overline{\uparrow\downarrow}}(k'', k''', q) \chi^{\omega'''\omega'\nu}_{0pp}(k''', k', q). \tag{11}$$

Within the DCA approximation, the single particle lattice self energy is coarse grained from its cluster counterpart, $\Sigma_\sigma(k, i\omega) = \Sigma_\sigma(K + \tilde{k}, i\omega) \approx \Sigma_\sigma(K, i\omega)$ and similarly the lattice susceptibility

$$\overline{\chi}^{\omega\omega'\nu}_{0pp}(K, K', Q) = \delta_{\omega\omega'} \delta_{kk'} \frac{N}{N_c} \sum_{\tilde{k}} G_\sigma(K + \tilde{k}, i\omega) G_\sigma(Q - K' + \tilde{k}, i\nu - i\omega'). \tag{12}$$

Also, according to Fotso *et al.* [2], using $\Gamma = \frac{\delta\Sigma}{\delta G}$, we can make the DCA substitution

$$\Gamma^{\omega\omega'\nu}_{pp\overline{\uparrow\downarrow}}(K, K', Q) = \Gamma^{\omega\omega'\nu}_{pp\overline{\uparrow\downarrow}}(K + \tilde{k}, K' + \tilde{k}', Q + \tilde{q}) \to \Gamma^{\omega\omega'\nu}_{cpp\overline{\uparrow\downarrow}}(K, K', Q). \tag{13}$$

We then sum over lattice momenta with one patch of k-space to get coarse-grain equation (11) as

$$\overline{\chi}^{\omega\omega'\nu}_{pp\overline{\uparrow\downarrow}}(K, K', Q) = \overline{\chi}^{\omega\omega'\nu}_{0pp}(K, K', Q) - \frac{1}{\beta^2} \overline{\chi}^{\omega\omega''\nu}_{pp\overline{\uparrow\downarrow}}(K, K'', Q) \Gamma^{\omega''\omega'''\nu}_{cpp\overline{\uparrow\downarrow}}(K'', K''', Q) \overline{\chi}^{\omega'''\omega'\nu}_{0pp}(K''', K', Q). \tag{14}$$

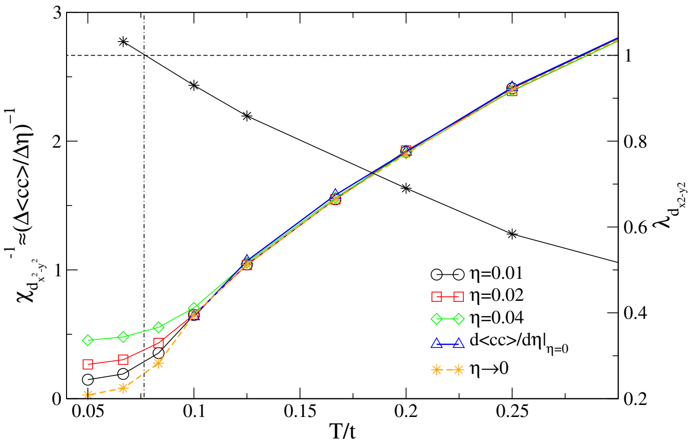


FIG. S1. Inverse $d_{x^2-y^2}$ superconducting susceptibility plotted against temperature for the two dimensional Hubbard model with $U = 8t$, next nearest neighbour hopping $t' = 0$ at chemical potential $\mu = -2$, using 2 by 2 cluster. Susceptibility obtained by measuring the response of order parameter with external $d$-wave field strength 0.01 (dashed line,circles black), 0.02 (dashed line, squares, red) and 0.04 (dashed line, diamonds, green). Susceptibility obtained by measuring 2-particle Green's function at normal state (solid line, triangle, blue). Also shown (right hand axis) the leading $d$-wave eigenvalue, $\lambda_{d_{x^2-y^2}}$, *vs* temperature.

Cluster quantities also follow the Bethe-salpeter equation,

$$\chi^{\omega\omega'\nu}_{cpp\overline{\uparrow\downarrow}}(K,K',Q) = \chi^{\omega\omega'\nu}_{0cpp}(K,K',Q) - \frac{1}{\beta^2}\chi^{\omega\omega''\nu}_{cpp\overline{\uparrow\downarrow}}(K,K'',Q)\Gamma^{\omega''\omega'''\nu}_{cpp\overline{\uparrow\downarrow}}(K'',K''',Q)\chi^{\omega'''\omega'\nu}_{c0pp}(K''',K',Q). \tag{15}$$

One then combines equations (14) and (15) to eliminate the cluster vertex, $\Gamma_c$, to obtain

$$\overline{\chi}^{-1} = \chi_c^{-1} - \chi_{0c}^{-1} + \overline{\chi}_0^{-1} \tag{16}$$

where $\overline{\chi}$, $\chi_c$, $\chi_{0c}$ and $\overline{\chi}_0$ are all matrices in cluster momentum $K$ and frequency $\omega$.
Equation (14) can also be written into a compact matrix form

$$\overline{\chi}_{pp\overline{\uparrow\downarrow}} = \frac{\overline{\chi}_0}{1 + \frac{1}{\beta^2}\Gamma_{cpp\overline{\uparrow\downarrow}}\overline{\chi}_0} \tag{17}$$

Finally, we define the correlated pairing susceptibility as the vertex part of the Bethe-Salpeter equation and include symmetry factors, giving,

$$\begin{aligned} P_g &:= (\chi - \chi_0)_g \\ &= \frac{1}{\beta^2}\sum_{\omega\omega' KK'} g(K)g(K')\left(\chi^{\omega\omega'\nu=0}_{pp\overline{\uparrow\downarrow}}(K,K',Q=0) - \chi_0^{\omega\omega'\nu=0}(K,K',Q=0)\right), \end{aligned} \tag{18}$$

where $g(K)$ is the coarse-grained symmetry factor.

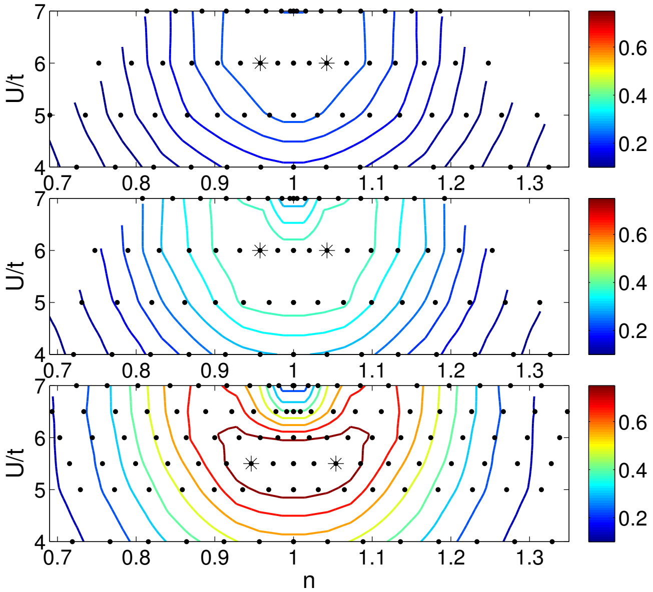


FIG. S2. Contour plot for $P_{d_{x^2-y^2}}$ in space of interaction strength and carrier concentration using 8-site cluster with no next nearest neighbour hopping. Top panel:$\beta = 7/t$; middle panel:$\beta = 10/t$; bottom panel:$\beta = 15/t$.

## VARIATION WITH TEMPERATURE AND CLUSTER SIZE

The procedure we detail in the main text operates under the assumption that the pair correlation function, susceptibilities and related eigenvalues have monotonic dependence with temperature. We show in Fig. S1 the consistent decrease of the inverse susceptibility with temperature. We find a correspondence between a downturn in inverse susceptibility with the eigenvalue of the $d_{x^2-y^2}$ channel passing through 1.

In Fig. S2 we demonstrate at $\beta t = 7$, 10 and 15, the evolution of $P_{d_{x^2-y^2}}$ for $N_c = 8$. We observe that the main features in $P_{d_{x^2-y^2}}$ does not much but the suppression near half filling is only observed below the pseudogap onset temperature.

We also explore the variation in system size in Fig. S3 for $N_c = 4$, 8, and 16 at temperatures $\beta t$ = 10, 15 and 5 respectively, which corresponds to $\approx 2T_c^{\max}$ for $N_c = 4, 8$ and $\approx 8T_c^{\max}$ for $N_c = 16$. We remark that larger clusters and lower temperatures are in principle accessible for some of the points presented in this phase diagram, but that the sign problem prevents us from showing an overview over the entire phase space for much lower $T$. For $N_c = 4$ the maximum in $P_{d_{x^2-y^2}}$ has been split into two along the line $n = 1$, due to the tendency of the $2 \times 2$ plaquette to form a Mott insulating phase at much weaker interaction than larger clusters (note that the physics of this cluster in DCA is different from the pseudogap physics observed on larger clusters, see, e.g., Refs. [4, 5]). We see that $N_c = 16$ contains no such artifact (similarly to $N_c = 8$). Further the structure near $n = 1$ is nearly identical in shape to the case of $N_c = 8$ for example, comparison to Fig. S2(a) shows the same structure.

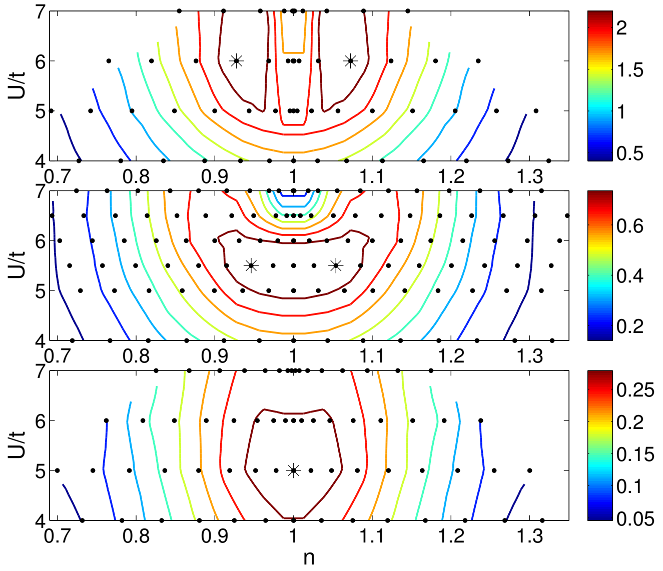


FIG. S3. The contour plot of $P_{d_{x^2-y^2}}$ in space of interaction strength and carrier concentration with only nearest neighbour hopping. Upper panel:4-site cluster, $\beta = 10/t$; middle panel: 8-site cluster, $\beta = 15/t$; bottom panel: 16-site cluster, $\beta = 5/t$.

Fig. S2 and S3 suggest that both reduction in temperature and increase in cluster size have an equivalent effect on the location of $\{U^{max}, n^{max}\}$, but the effect appears primarily as a shift in $U^{max}$, to a lower value, and not as a change in optimal density, $n^{max}$. Convergence of these finite size effects will require larger clusters but has been done for $T_c$ on clusters with about twice the size considered here [6].

## WEAK COUPLING

We expand upon the exploration of symmetries in the main text, by examining the doping dependence of the superconducting order symmetry in the weak coupling regime. In Figs. S4 and S5 we examine the case of $U/t = 2$, a weakly coupled case, which has been suggested by recent weak coupling work to show a transition from $p-$wave to $d_{xy}$ to $d_{x^2-y^2}$ [7].

We find from examining the leading eigenvalue at two temperatures, $\beta = 15$ and 33, that in the $n = 2$ limit has a weakly dominant $p$-wave component, which gives way to $d_{xy}$ and then $d_{x^2-y^2}$ as number density is decreased towards half filling. However, in the case of $d_{xy}$ symmetry, there is essentially no temperature dependence in the eigenvalue, suggesting no clear proximity to a divergence in this eigenvalue at the temperature examined, despite being the dominant channel. This is contrasted by the same temperature change, and it's effect on $\lambda_{d_{x^2-y^2}}$ which shows rather substantial temperature changes. Similarly the $p-$wave eigenvalue near $n = 2$ changes somewhat with $\beta$ (though any $T_c$ would be far below the temperatures accessible in this simulation).

At $n = 1.75$, the leading eigenvalue of the system has $d_{xy}$ symmetry (Fig. S4) but is very far away

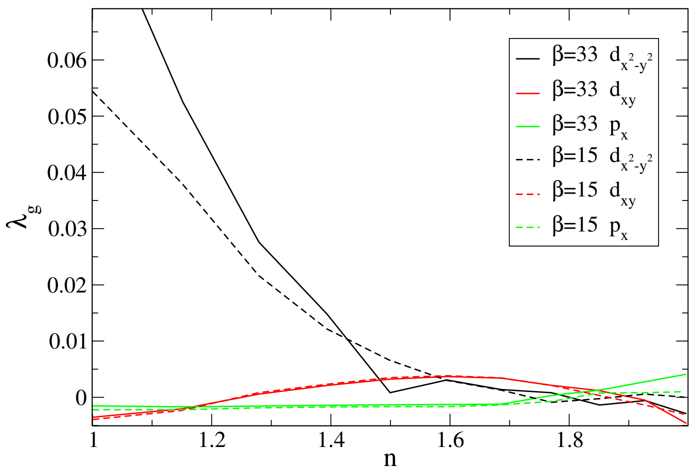


FIG. S4. The leading eigenvalue, $\lambda_g$, in each of $x^2 - y^2$, $xy$, and $p$ channels for $U/t = 2$ at $\beta t = 15$ (dashed) and $\beta t = 33$ (solid).

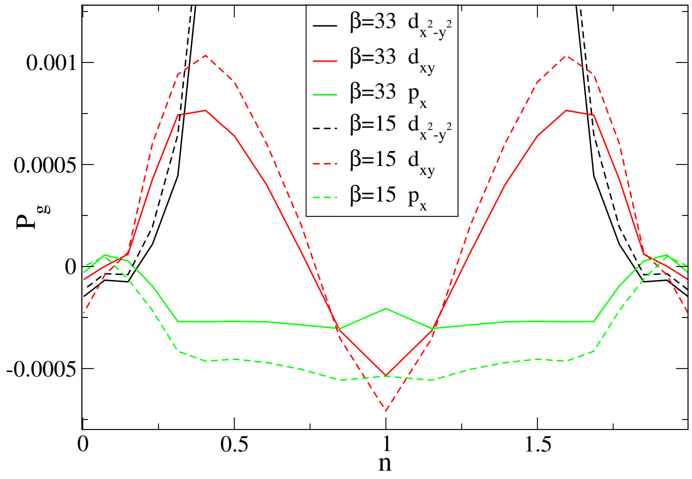


FIG. S5. The correlated pairing susceptibility, $P_g$, in each of $x^2 - y^2$, $xy$, and $p$ channels for $U/t = 2$ at $\beta t = 33$(solid).

from 1. For the same parameters, the correlated pairing susceptibility, shown in Fig. S5, similarly has a dominant contribution but is far away from a divergence. Decreasing temperature reduces the value of $P_{d_{xy}}$ rather than increasing it as would be expected on approach to a transition to a $d_{xy}$ order.

[1] G. Rohringer, A. Valli, and A. Toschi, Phys. Rev. B **86**, 125114 (2012), arXiv:1202.2796 [cond-mat.str-el].
[2] H. Fotso, S. Yang, K. Chen, S. Pathak, J. Moreno, M. Jarrell, K. Mikelsons, E. Khatami, and D. Galanakis, *Dynamical Cluster Approximation* (Springer-Verlag Berlin Heidelberg, 2012).
[3] E. Khatami, R. T. Scalettar, and R. R. P. Singh, Phys. Rev. B **91**, 241107 (2015).
[4] E. Gull, P. Werner, X. Wang, M. Troyer, and A. J. Millis, EPL (Europhysics Letters) **84**, 37009 (2008).
[5] E. Gull, M. Ferrero, O. Parcollet, A. Georges, and A. J. Millis, Phys. Rev. B **82**, 155101 (2010).
[6] T. A. Maier, M. Jarrell, T. C. Schulthess, P. R. C. Kent, and J. B. White, Phys. Rev. Lett. **95**, 237001 (2005).
[7] Y. Deng, E. Kozik, N. V. Prokof'ev, and B. V. Svistunov, EPL (Europhysics Letters) **110**, 57001 (2015).
